# Supplementary material for: Cerberus: A Formal Approach to Secure and Efficient Enclave Memory Sharing
Source: arXiv:2209.15253 source file (2022-11-14)
Supplement: Supplementary file 1 [file appendix.tex]

\newpage
\clearpage
\label{appendix}
\section*{\appendixname}

\begin{table}[!htb]
    \centering
    \begin{minipage}{\textwidth}
        \begin{tabular}[t]{ p{0.15\textwidth} p{0.75\textwidth} }
        \specialrule{.1em}{.1em}{.1em}
        \textbf{Symbol} & \textbf{Description}\\
        \hline
        $\mathbb{N}$ & The usual set of natural numbers $\{ 1, 2, 3, ... \}$.\\
        \textit{Bool} & The set of Boolean values $\{\textit{true}, \textit{false}\}$.\\
        \hline
        $\in$ & \textit{Element of} operator in set theory.\\
        $\subset$ & Subset operator.\\
        $\cup$ & Set union operator.\\
        $\{\cdot\}$ & The singleton set. \\

        $\stackrel{.}{=}$ & \textit{By definition} symbol. This is not to be confused with the logical equal operator $=$. \\
        $=$ & Logical equal operator. \\
        $\iff$ & If and only if operator. \\
        $\land$ & Logical conjunction. \\
        $\lor$ & Logical disjunction. \\
        $\neg$ & Logical negation. \\

        \hline
        $\bot$ & Bottom value. A default value that is only equal to itself.\\
        $\mathcal{OS}$ & The identifier for the enclave.\\
        $\textit{e}_{inv}$ & The invalid enclave ID. A variable assigned with this ID can be viewed as a null value.\\
        \hline
        $\VA$ & Set of virtual addresses.\\
        $\PA$ & Set of physical addresses.\\
        $ACL$ & Permissions for virtual addresses (read, write and execute permissions).\\
        $\mathcal{E}_{id}$ & Set of enclave IDs $e_1, e_2, ...$, including the operating system ID $\mathcal{OS}$.\\
        $\mathcal{E}_M$ & Enclave metadata type.\\
        \hline
        $\forall x\in X.expr(x)$ & Forall quantified expression; states for all $x\in X$, $expr(x)$ must be true.\\
        $\lambda x.expr$ & Function with argument $x$; computes $expr$.\\
        $\textit{ITE}(c, expr_1, expr_2)$ & If-then-else operator that evaluates $expr_1$ if $c$ is true or otherwise evaluates $expr_2$.\\
        $\textit{init}(E_e(\sigma))$ & Enclave $e$ in state $\sigma$ has been initialized by $\launchop$ and has not yet been executed using $\enterop$.\\
        $\textit{sufficient\_mem}(\sigma.\towner)$ & A function that returns whether there is enough memory to allocate given the memory ownership map.\\
        $\textit{valid}(e_{id})$ & Returns whether the enclave ID $e_{id}$ is a valid enclave ID. A valid enclave ID is not equal to $\mathcal{OS}$ nor $e_{inv}$.\\
        $\textit{active}(e_{id}, \sigma)$ & Returns true if and only if the enclave with ID $e_{id}$ has been launched or cloned and is not yet destroyed.\\
        $\textit{mapped}_e(v)$ & Returns whether a virtual address $v\in\VA$ is mapped for the enclave $e$.\\
        $\textit{curr}(\sigma)$ & The ID of the process currently executing in state $\sigma$.\\
        \hline
        $S$ & Set of state of \tapc.\\
        $S\times S$ & Set of pairs of states of \tapc. The $\times$ operator is the usual Cartesian product.\\
        $I$ & Set of initial states of \tapc.\\
        $\rightsquigarrow$ & Transition relation of \tapc.\\
        $E_e(\sigma)$ & The projection of state $\sigma$ to the enclave state $e$.\\
        $A_e(\sigma)$ & The projection of state $\sigma$ to state that is writable to the adversary.\\
        $I_e(\sigma)$ & Inputs of an enclave at state $\sigma$.\\
        $O_e(\sigma)$ & Outputs of an enclave at state $\sigma$.\\
        \hline
        $\pi^i$ & The $i$th state of the platform trace $\pi$.\\
        $\pi_j$ & Platform trace $j$; not to be confused with the $j$th state of the trace.\\
        \specialrule{.1em}{.1em}{.1em}
        \end{tabular}
    \end{minipage}
    \caption{\textbf{Glossary of Symbols}}
    \label{fig:glossary}
\end{table}
